# Supplementary material for: Semantic, Efficient, and Secure Search over Encrypted Cloud Data
Source: arXiv:2002.10294 source file (2020-02-24)
Supplement: Supplementary file 1 [file appendix1.tex]

%%%%%%%%%%%%%%%%%%%%%%%%%%%%%%%%%%%%%%%%%%%%%%%%%%%%%%%%%%%%%%%%%%%%%%%%%%%%%%%%
%2345678901234567890123456789012345678901234567890123456789012345678901234567890
%        1         2         3         4         5         6         7         8
% THESIS APPENDIX

\chapter{Gesture Vocabulary} 
\label{chap:appendixA}

\begin{figure}
    \centering
    \includegraphics[width=0.8\textwidth]{Chapter4/Figures/Figures/gv.PNG}
    \caption{Proposed gesture vocabulary}
    \label{fig:gs}
\end{figure}
