# Supplementary material for: Semantic, Efficient, and Secure Search over Encrypted Cloud Data
Source: arXiv:2002.10294 source file (2020-02-24)
Supplement: Supplementary file 2 [file appendix2.tex]

\chapter{Survey}
\label{chap:appendixB}

%\begin{figure}
%\setboolean{@twoside}{false}
% Uncomment the follow line to show the survey
\includepdf[pages=1-,scale=0.8,pagecommand={}]{Appendix2/gbhri3_format.pdf}
%\end{figure}

%\begin{figure}
 %\centering 
 %\includegraphics{Appendix2/gbhri3_format.pdf}
%\end{figure}
